# Supplementary material for: Ion Impact Induced Ultrafast Electron Dynamics in Correlated Materials and Finite Graphene Clusters
Source: arXiv:1808.07868 source file (2018-09-19)
Supplement: Supplementary file 2 [file test1.tex]

%% test1.tex
%%
%% This is file `test1.tex', one of a set of several test/example files
%% in the `subfig' package.
%%
%% Copyright © 2003, 2004, 2005 Steven Douglas Cochran.
%% 
%% This work (the subfig package) may be distributed and/or modified 
%% under the conditions of the LaTeX Project Public License, either 
%% version 1.3 of this license or (at your option) any later version.
%% The latest version of this license is in
%%   http://www.latex-project.org/lppl.txt
%% and version 1.3 or later is part of all distributions of LaTeX
%% version 2003/12/01 or later.
%%
%% This work has the LPPL maintenance status "author-maintained".
%% 
%% This Current Maintainer of this work is Steven Douglas Cochran.
%%
%% This work consists of all files listed under "MANIFEST" in the
%% README file distributed with the subfig package.

\documentclass[twocolumn]{article}

\usepackage{caption}
\usepackage[labelfont=bf,textfont={sl,bf},lofdepth,lotdepth]{subfig}
\DeclareCaptionListOfFormat{colon}{#2:}
\usepackage{fixltx2e}

\captionsetup[subtable]{listofformat=colon,listofnumwidth=1.5em,
                        listofindent=3.8em}
\newcommand{\figbox}[1]{%
  \fbox{%
    \vbox to 1in{%
    \vfil
    \hbox to 2in{%
      \hfil
      #1%
      \hfil}%
    \vfil}}}

\makeatletter
  \newcommand{\setcaptype}[1]{%
    \listsubcaptions
    \renewcommand{\@captype}{#1}}
  \renewcommand\abstract[1]{%
    \def\@abstract{%
      \centerline{{\large\bf Abstract}}
      \noindent
      #1}}
  \renewcommand\@maketitle{%
    \newpage
    \null\vfil
    \vskip 60\p@
    \begin{center}%
      {\LARGE \@title \par}%
      \vskip 3em%
      {\large
       \lineskip .75em%
       \begin{tabular}[t]{c}%
         \@author
       \end{tabular}\par}%
      \vskip 1.5em%
      {\large \@date \par}% 
    \end{center}%
    \vskip 2.5em%
    \@abstract
    \vfil\null}%
\makeatother

\begin{document}

\title{Subfig Package Test Program One}
\author{Steven Douglas Cochran\\
        Digital Mapping Laboratory\\
        School of Computer Science\\
        Carnegie-Mellon University\\
        5000 Forbes Avenue\\
        Pittsburgh, PA 15213-3890\\
        USA}
\date{21 December 2003}
\abstract{%
This test checks five things:
\begin{enumerate}
  \item if the {\bf subfig} and the {\bf fixltx2e} packages work together;
  \item that the subcaption label format for the List-of-Float pages
        is working;
  \item that the subcaption numbering in the List-of-Float pages is
        working;
  \item it tests the {\bf figure*} and {\bf table*} environemnts in 
        two column mode; and,
  \item that various position combinations of top and bottom captions and 
        subcaptions work together.
\end{enumerate}}
\maketitle
\clearpage

\listoffigures
\clearpage

\listoftables
\clearpage

\section{Overview}

This test runs through the various layout options for both figures and
subfigures; and tables and subtables.  It also shows a mixture of
figures and tables within a single float environment.

\subsection{Multiple figures}
\captionsetup[figure]{position=bottom}
\captionsetup[table]{position=bottom}

Figure~\ref{fig:Afirst}[\pageref{fig:Afirst}] has two subfigures
\ref{fig:AfirstA}[\pageref{fig:AfirstA}] and
\ref{fig:AfirstB}[\pageref{fig:AfirstB}].
%
Figure~\ref{fig:Asecond}[\pageref{fig:Asecond}] has two subfigures
\ref{fig:AsecondA}[\pageref{fig:AsecondA}] and
\ref{fig:AsecondB}[\pageref{fig:AsecondB}].
%
Figure~\ref{fig:Athird}[\pageref{fig:Athird}] has two subfigures
\ref{fig:AthirdA}[\pageref{fig:AthirdA}] and
\ref{fig:AthirdB}[\pageref{fig:AthirdB}].
%
Figure~\ref{fig:Afourth}[\pageref{fig:Afourth}] has two subfigures
\ref{fig:AfourthA}[\pageref{fig:AfourthA}] and
\ref{fig:AfourthB}[\pageref{fig:AfourthB}].
%
Figure~\ref{fig:Afifth}[\pageref{fig:Afifth}] has two subfigures
\ref{fig:AfifthA}[\pageref{fig:AfifthA}] and
\ref{fig:AfifthB}[\pageref{fig:AfifthB}].
%
Figure~\ref{fig:Asixth}[\pageref{fig:Asixth}] has two subfigures
\ref{fig:AsixthA}[\pageref{fig:AsixthA}] and
\ref{fig:AsixthB}[\pageref{fig:AsixthB}].

\begin{figure*}%
    \captionsetup[figure]{margin=10pt}%
    \subfloat[One subone.\label{fig:AfirstA}]{\figbox{One subone}}
    \hfill
    \subfloat[One subtwo.\label{fig:AfirstB} --- but this one has a
     very very long caption.  So long that it continues over into 
     other lines so that we can test the list-of line settings.]%
     {\figbox{One subtwo}}\\[-10pt]
    \caption{First figure --- but this one has a very very long caption.
     So long that it continues over into a second line so that we can 
     test the margin setting and centering of the caption command in the
     full page mode.}%
    \label{fig:Afirst}%
%
    \subfloat[Two subone.\label{fig:AsecondA}]{\figbox{Two subone}}
    \hfill
    \subfloat[Two subtwo.\label{fig:AsecondB}]{\figbox{Two subtwo}}\\[-10pt]
    \caption{Second figure.}%
    \label{fig:Asecond}%
%
    \subfloat[Three subone.\label{fig:AthirdA}]{\figbox{Three subone}}
    \hfill
    \subfloat[Three subtwo.\label{fig:AthirdB}]{\figbox{Three subtwo}}\\[-10pt]
    \caption{Third figure.}%
    \label{fig:Athird}%
\end{figure*}

\begin{figure*}%
  \begin{center}%
    \subfloat[Four subone.\label{fig:AfourthA}]{\figbox{Four subone}}
    \qquad
    \subfloat[Four subtwo.\label{fig:AfourthB}]{\figbox{Four subtwo}}\\[-10pt]
    \caption{Fourth figure.}%
    \label{fig:Afourth}%
%
    \subfloat[Five subone.\label{fig:AfifthA}]{\figbox{Five subone}}
    \qquad
    \subfloat[Five subtwo.\label{fig:AfifthB}]{\figbox{Five subtwo}}\\[-10pt]
    \caption{Fifth figure.}%
    \label{fig:Afifth}%
%
    \subfloat[Six subone.\label{fig:AsixthA}]{\figbox{Six subone}}
    \qquad
    \subfloat[Six subtwo.\label{fig:AsixthB}]{\figbox{Six subtwo}}\\[-10pt]
    \caption{Sixth figure.}%
    \label{fig:Asixth}%
  \end{center}
\end{figure*}

\subsection{Multiple tables}

Table~\ref{tab:Afirst}[\pageref{tab:Afirst}] has two subtables
\ref{tab:AfirstA}[\pageref{tab:AfirstA}] and
\ref{tab:AfirstB}[\pageref{tab:AfirstB}].
%
Table~\ref{tab:Asecond}[\pageref{tab:Asecond}] has two subtables
\ref{tab:AsecondA}[\pageref{tab:AsecondA}] and
\ref{tab:AsecondB}[\pageref{tab:AsecondB}].
%
Table~\ref{tab:Athird}[\pageref{tab:Athird}] has two subtables
\ref{tab:AthirdA}[\pageref{tab:AthirdA}] and
\ref{tab:AthirdB}[\pageref{tab:AthirdB}].
%
Table~\ref{tab:Afourth}[\pageref{tab:Afourth}] has two subtables
\ref{tab:AfourthA}[\pageref{tab:AfourthA}] and
\ref{tab:AfourthB}[\pageref{tab:AfourthB}].
%
Table~\ref{tab:Afifth}[\pageref{tab:Afifth}] has two subtables
\ref{tab:AfifthA}[\pageref{tab:AfifthA}] and
\ref{tab:AfifthB}[\pageref{tab:AfifthB}].
%
Table~\ref{tab:Asixth}[\pageref{tab:Asixth}] has two subtables
\ref{tab:AsixthA}[\pageref{tab:AsixthA}] and
\ref{tab:AsixthB}[\pageref{tab:AsixthB}].

\begin{table*}%
  \begin{center}%
    \subfloat[One subone.\label{tab:AfirstA}]{\figbox{One subone}}
    \qquad
    \subfloat[One subtwo.\label{tab:AfirstB}]{\figbox{One subtwo}}\\[-10pt]
    \caption{First table.}%
    \label{tab:Afirst}%
%
    \subfloat[Two subone.\label{tab:AsecondA}]{\figbox{Two subone}}
    \qquad
    \subfloat[Two subtwo.\label{tab:AsecondB}]{\figbox{Two subtwo}}\\[-10pt]
    \caption{Second table.}%
    \label{tab:Asecond}%
%
    \subfloat[Three subone.\label{tab:AthirdA}]{\figbox{Three subone}}
    \qquad
    \subfloat[Three subtwo.\label{tab:AthirdB}]{\figbox{Three subtwo}}\\[-10pt]
    \caption{Third table.}%
    \label{tab:Athird}%
  \end{center}%
\end{table*}

\begin{table*}%
  \begin{center}%
    \subfloat[Four subone.\label{tab:AfourthA}]{\figbox{Four subone}}
    \qquad
    \subfloat[Four subtwo.\label{tab:AfourthB}]{\figbox{Four subtwo}}\\[-10pt]
    \caption{Fourth table.}%
    \label{tab:Afourth}%
%
    \subfloat[Five subone.\label{tab:AfifthA}]{\figbox{Five subone}}
    \qquad
    \subfloat[Five subtwo.\label{tab:AfifthB}]{\figbox{Five subtwo}}\\[-10pt]
    \caption{Fifth table.}%
    \label{tab:Afifth}%
%
    \subfloat[Six subone.\label{tab:AsixthA}]{\figbox{Six subone}}
    \qquad
    \subfloat[Six subtwo.\label{tab:AsixthB}]{\figbox{Six subtwo}}\\[-10pt]
    \caption{Sixth table.}%
    \label{tab:Asixth}%
  \end{center}%
\end{table*}

\subsection{Multiple figures with the {\bf figure} caption at top}
\captionsetup[figure]{position=top}

Figure~\ref{fig:Bfirst}[\pageref{fig:Bfirst}] has two subfigures
\ref{fig:BfirstA}[\pageref{fig:BfirstA}] and
\ref{fig:BfirstB}[\pageref{fig:BfirstB}].
%
Figure~\ref{fig:Bsecond}[\pageref{fig:Bsecond}] has two subfigures
\ref{fig:BsecondA}[\pageref{fig:BsecondA}] and
\ref{fig:BsecondB}[\pageref{fig:BsecondB}].
%
Figure~\ref{fig:Bthird}[\pageref{fig:Bthird}] has two subfigures
\ref{fig:BthirdA}[\pageref{fig:BthirdA}] and
\ref{fig:BthirdB}[\pageref{fig:BthirdB}].
%
Figure~\ref{fig:Bfourth}[\pageref{fig:Bfourth}] has two subfigures
\ref{fig:BfourthA}[\pageref{fig:BfourthA}] and
\ref{fig:BfourthB}[\pageref{fig:BfourthB}].
%
Figure~\ref{fig:Bfifth}[\pageref{fig:Bfifth}] has two subfigures
\ref{fig:BfifthA}[\pageref{fig:BfifthA}] and
\ref{fig:BfifthB}[\pageref{fig:BfifthB}].
%
Figure~\ref{fig:Bsixth}[\pageref{fig:Bsixth}] has two subfigures
\ref{fig:BsixthA}[\pageref{fig:BsixthA}] and
\ref{fig:BsixthB}[\pageref{fig:BsixthB}].

\begin{figure*}%
  \begin{center}%
    \caption{First figure.}%
    \label{fig:Bfirst}%
    \subfloat[One subone.\label{fig:BfirstA}]{\figbox{One subone}}
    \qquad
    \subfloat[One subtwo.\label{fig:BfirstB}]{\figbox{One subtwo}}\\
%
    \caption{Second figure.}%
    \label{fig:Bsecond}%
    \subfloat[Two subone.\label{fig:BsecondA}]{\figbox{Two subone}}
    \qquad
    \subfloat[Two subtwo.\label{fig:BsecondB}]{\figbox{Two subtwo}}\\
%
    \caption{Third figure.}%
    \label{fig:Bthird}%
    \subfloat[Three subone.\label{fig:BthirdA}]{\figbox{Three subone}}
    \qquad
    \subfloat[Three subtwo.\label{fig:BthirdB}]{\figbox{Three subtwo}}%
  \end{center}%
\end{figure*}

\begin{figure*}%
  \begin{center}%
    \caption{Fourth figure.}%
    \label{fig:Bfourth}%
    \subfloat[Four subone.\label{fig:BfourthA}]{\figbox{Four subone}}
    \qquad
    \subfloat[Four subtwo.\label{fig:BfourthB}]{\figbox{Four subtwo}}\\
%
    \caption{Fifth figure.}%
    \label{fig:Bfifth}%
    \subfloat[Five subone.\label{fig:BfifthA}]{\figbox{Five subone}}
    \qquad
    \subfloat[Five subtwo.\label{fig:BfifthB}]{\figbox{Five subtwo}}\\
%
    \caption{Sixth figure.}%
    \label{fig:Bsixth}%
    \subfloat[Six subone.\label{fig:BsixthA}]{\figbox{Six subone}}
    \qquad
    \subfloat[Six subtwo.\label{fig:BsixthB}]{\figbox{Six subtwo}}
  \end{center}%
\end{figure*}

\subsection{Multiple tables with the {\bf table} caption at top}
\captionsetup[table]{position=top}

Table~\ref{tab:Bfirst}[\pageref{tab:Bfirst}] has two subtables
\ref{tab:BfirstA}[\pageref{tab:BfirstA}] and
\ref{tab:BfirstB}[\pageref{tab:BfirstB}].
%
Table~\ref{tab:Bsecond}[\pageref{tab:Bsecond}] has two subtables
\ref{tab:BsecondA}[\pageref{tab:BsecondA}] and
\ref{tab:BsecondB}[\pageref{tab:BsecondB}].
%
Table~\ref{tab:Bthird}[\pageref{tab:Bthird}] has two subtables
\ref{tab:BthirdA}[\pageref{tab:BthirdA}] and
\ref{tab:BthirdB}[\pageref{tab:BthirdB}].
%
Table~\ref{tab:Bfourth}[\pageref{tab:Bfourth}] has two subtables
\ref{tab:BfourthA}[\pageref{tab:BfourthA}] and
\ref{tab:BfourthB}[\pageref{tab:BfourthB}].
%
Table~\ref{tab:Bfifth}[\pageref{tab:Bfifth}] has two subtables
\ref{tab:BfifthA}[\pageref{tab:BfifthA}] and
\ref{tab:BfifthB}[\pageref{tab:BfifthB}].
%
Table~\ref{tab:Bsixth}[\pageref{tab:Bsixth}] has two subtables
\ref{tab:BsixthA}[\pageref{tab:BsixthA}] and
\ref{tab:BsixthB}[\pageref{tab:BsixthB}].

\begin{table*}%
  \begin{center}%
    \caption{First table.}%
    \label{tab:Bfirst}%
    \subfloat[One subone.\label{tab:BfirstA}]{\figbox{One subone}}
    \qquad
    \subfloat[One subtwo.\label{tab:BfirstB}]{\figbox{One subtwo}}\\
%
    \caption{Second table.}%
    \label{tab:Bsecond}%
    \subfloat[Two subone.\label{tab:BsecondA}]{\figbox{Two subone}}
    \qquad
    \subfloat[Two subtwo.\label{tab:BsecondB}]{\figbox{Two subtwo}}\\
%
    \caption{Third table.}%
    \label{tab:Bthird}%
    \subfloat[Three subone.\label{tab:BthirdA}]{\figbox{Three subone}}
    \qquad
    \subfloat[Three subtwo.\label{tab:BthirdB}]{\figbox{Three subtwo}}\\
  \end{center}%
\end{table*}

\begin{table*}%
  \begin{center}%
    \caption{Fourth table.}%
    \label{tab:Bfourth}%
    \subfloat[Four subone.\label{tab:BfourthA}]{\figbox{Four subone}}
    \qquad
    \subfloat[Four subtwo.\label{tab:BfourthB}]{\figbox{Four subtwo}}
%
    \caption{Fifth table.}%
    \label{tab:Bfifth}%
    \subfloat[Five subone.\label{tab:BfifthA}]{\figbox{Five subone}}
    \qquad
    \subfloat[Five subtwo.\label{tab:BfifthB}]{\figbox{Five subtwo}}
%
    \caption{Sixth table.}%
    \label{tab:Bsixth}%
    \subfloat[Six subone.\label{tab:BsixthA}]{\figbox{Six subone}}
    \qquad
    \subfloat[Six subtwo.\label{tab:BsixthB}]{\figbox{Six subtwo}}
  \end{center}%
\end{table*}


\subsection{Multiple figures with the {\bf figure} and {\bf subfigure}
            captions at top}
\captionsetup[subfigure]{position=top}

Figure~\ref{fig:Cfirst}[\pageref{fig:Cfirst}] has two subfigures
\ref{fig:CfirstA}[\pageref{fig:CfirstA}] and
\ref{fig:CfirstB}[\pageref{fig:CfirstB}].
%
Figure~\ref{fig:Csecond}[\pageref{fig:Csecond}] has two subfigures
\ref{fig:CsecondA}[\pageref{fig:CsecondA}] and
\ref{fig:CsecondB}[\pageref{fig:CsecondB}].
%
Figure~\ref{fig:Cthird}[\pageref{fig:Cthird}] has two subfigures
\ref{fig:CthirdA}[\pageref{fig:CthirdA}] and
\ref{fig:CthirdB}[\pageref{fig:CthirdB}].
%
Figure~\ref{fig:Cfourth}[\pageref{fig:Cfourth}] has two subfigures
\ref{fig:CfourthA}[\pageref{fig:CfourthA}] and
\ref{fig:CfourthB}[\pageref{fig:CfourthB}].
%
Figure~\ref{fig:Cfifth}[\pageref{fig:Cfifth}] has two subfigures
\ref{fig:CfifthA}[\pageref{fig:CfifthA}] and
\ref{fig:CfifthB}[\pageref{fig:CfifthB}].
%
Figure~\ref{fig:Csixth}[\pageref{fig:Csixth}] has two subfigures
\ref{fig:CsixthA}[\pageref{fig:CsixthA}] and
\ref{fig:CsixthB}[\pageref{fig:CsixthB}].

\begin{figure*}%
  \begin{center}%
    \caption{First figure.}%
    \label{fig:Cfirst}%
    \subfloat[One subone.\label{fig:CfirstA}]{\figbox{One subone}}
    \qquad
    \subfloat[One subtwo.\label{fig:CfirstB}]{\figbox{One subtwo}}\\
%
    \caption{Second figure.}%
    \label{fig:Csecond}%
    \subfloat[Two subone.\label{fig:CsecondA}]{\figbox{Two subone}}
    \qquad
    \subfloat[Two subtwo.\label{fig:CsecondB}]{\figbox{Two subtwo}}\\
%
    \caption{Third figure.}%
    \label{fig:Cthird}%
    \subfloat[Three subone.\label{fig:CthirdA}]{\figbox{Three subone}}
    \qquad
    \subfloat[Three subtwo.\label{fig:CthirdB}]{\figbox{Three subtwo}}\\
  \end{center}%
\end{figure*}

\begin{figure*}%
  \begin{center}%
    \caption{Fourth figure.}%
    \label{fig:Cfourth}%
    \subfloat[Four subone.\label{fig:CfourthA}]{\figbox{Four subone}}
    \qquad
    \subfloat[Four subtwo.\label{fig:CfourthB}]{\figbox{Four subtwo}}\\
%
    \caption{Fifth figure.}%
    \label{fig:Cfifth}%
    \subfloat[Five subone.\label{fig:CfifthA}]{\figbox{Five subone}}
    \qquad
    \subfloat[Five subtwo.\label{fig:CfifthB}]{\figbox{Five subtwo}}\\
%
    \caption{Sixth figure.}%
    \label{fig:Csixth}%
    \subfloat[Six subone.\label{fig:CsixthA}]{\figbox{Six subone}}
    \qquad
    \subfloat[Six subtwo.\label{fig:CsixthB}]{\figbox{Six subtwo}}\\
  \end{center}%
\end{figure*}

\subsection{Multiple tables with the {\bf table} and {\bf subtable}
            captions at top}
\captionsetup[subtable]{position=top}

Table~\ref{tab:Cfirst}[\pageref{tab:Cfirst}] has two subtables
\ref{tab:CfirstA}[\pageref{tab:CfirstA}] and
\ref{tab:CfirstB}[\pageref{tab:CfirstB}].
%
Table~\ref{tab:Csecond}[\pageref{tab:Csecond}] has two subtables
\ref{tab:CsecondA}[\pageref{tab:CsecondA}] and
\ref{tab:CsecondB}[\pageref{tab:CsecondB}].
%
Table~\ref{tab:Cthird}[\pageref{tab:Cthird}] has two subtables
\ref{tab:CthirdA}[\pageref{tab:CthirdA}] and
\ref{tab:CthirdB}[\pageref{tab:CthirdB}].
%
Table~\ref{tab:Cfourth}[\pageref{tab:Cfourth}] has two subtables
\ref{tab:CfourthA}[\pageref{tab:CfourthA}] and
\ref{tab:CfourthB}[\pageref{tab:CfourthB}].
%
Table~\ref{tab:Cfifth}[\pageref{tab:Cfifth}] has two subtables
\ref{tab:CfifthA}[\pageref{tab:CfifthA}] and
\ref{tab:CfifthB}[\pageref{tab:CfifthB}].
%
Table~\ref{tab:Csixth}[\pageref{tab:Csixth}] has two subtables
\ref{tab:CsixthA}[\pageref{tab:CsixthA}] and
\ref{tab:CsixthB}[\pageref{tab:CsixthB}].

\begin{table*}%
  \begin{center}%
    \caption{First table.}%
    \label{tab:Cfirst}%
    \subfloat[One subone.\label{tab:CfirstA}]{\figbox{One subone}}
    \qquad
    \subfloat[One subtwo.\label{tab:CfirstB}]{\figbox{One subtwo}}\\
%
    \caption{Second table.}%
    \label{tab:Csecond}%
    \subfloat[Two subone.\label{tab:CsecondA}]{\figbox{Two subone}}
    \qquad
    \subfloat[Two subtwo.\label{tab:CsecondB}]{\figbox{Two subtwo}}\\
%
    \caption{Third table.}%
    \label{tab:Cthird}%
    \subfloat[Three subone.\label{tab:CthirdA}]{\figbox{Three subone}}
    \qquad
    \subfloat[Three subtwo.\label{tab:CthirdB}]{\figbox{Three subtwo}}\\
  \end{center}%
\end{table*}

\begin{table*}%
  \begin{center}%
    \caption{Fourth table.}%
    \label{tab:Cfourth}%
    \subfloat[Four subone.\label{tab:CfourthA}]{\figbox{Four subone}}
    \qquad
    \subfloat[Four subtwo.\label{tab:CfourthB}]{\figbox{Four subtwo}}\\
%
    \caption{Fifth table.}%
    \label{tab:Cfifth}%
    \subfloat[Five subone.\label{tab:CfifthA}]{\figbox{Five subone}}
    \qquad
    \subfloat[Five subtwo.\label{tab:CfifthB}]{\figbox{Five subtwo}}\\
%
    \caption{Sixth table.}%
    \label{tab:Csixth}%
    \subfloat[Six subone.\label{tab:CsixthA}]{\figbox{Six subone}}
    \qquad
    \subfloat[Six subtwo.\label{tab:CsixthB}]{\figbox{Six subtwo}}\\
  \end{center}%
\end{table*}

\subsection{Mixed figures and tables with only the {\bf table} caption
            at top}
\captionsetup[figure]{position=bottom}
%\setcounter{subfigure}{0}
\captionsetup[subfigure]{position=bottom}
\captionsetup[table]{position=top}
%\setcounter{subtable}{0}
\captionsetup[subtable]{position=bottom}

Figure~\ref{fig:Dfirst}[\pageref{fig:Dfirst}] has two subfigures
\ref{fig:DfirstA}[\pageref{fig:DfirstA}] and
\ref{fig:DfirstB}[\pageref{fig:DfirstB}].
%
Table~\ref{tab:Dfirst}[\pageref{tab:Dfirst}] has two subtables
\ref{tab:DfirstA}[\pageref{tab:DfirstA}] and
\ref{tab:DfirstB}[\pageref{tab:DfirstB}].
%
Figure~\ref{fig:Dsecond}[\pageref{fig:Dsecond}] has two subfigures
\ref{fig:DsecondA}[\pageref{fig:DsecondA}] and
\ref{fig:DsecondB}[\pageref{fig:DsecondB}].
%
Figure~\ref{fig:Dthird}[\pageref{fig:Dthird}] has two subfigures
\ref{fig:DthirdA}[\pageref{fig:DthirdA}] and
\ref{fig:DthirdB}[\pageref{fig:DthirdB}].
%
Table~\ref{tab:Dsecond}[\pageref{tab:Dsecond}] has two subtables
\ref{tab:DsecondA}[\pageref{tab:DsecondA}] and
\ref{tab:DsecondB}[\pageref{tab:DsecondB}].
%
Table~\ref{tab:Dthird}[\pageref{tab:Dthird}] has two subtables
\ref{tab:DthirdA}[\pageref{tab:DthirdA}] and
\ref{tab:DthirdB}[\pageref{tab:DthirdB}].

\begin{figure*}%
  \begin{center}%
    \subfloat[One subone.\label{fig:DfirstA}]{\figbox{One subone}}
    \qquad
    \subfloat[One subtwo.\label{fig:DfirstB}]{\figbox{One subtwo}}\\[-10pt]
    \caption{First figure.}%
    \label{fig:Dfirst}%
%
    \setcaptype{table}%
    \caption{First table.}%
    \label{tab:Dfirst}%
    \subfloat[One subone.\label{tab:DfirstA}]{\figbox{One subone}}
    \qquad
    \subfloat[One subtwo.\label{tab:DfirstB}]{\figbox{One subtwo}}\\
    \listsubcaptions
%
    \setcaptype{figure}%
    \subfloat[Two subone.\label{fig:DsecondA}]{\figbox{Two subone}}
    \qquad
    \subfloat[Two subtwo.\label{fig:DsecondB}]{\figbox{Two subtwo}}\\[-10pt]
    \caption{Second figure.}%
    \label{fig:Dsecond}%
  \end{center}%
\end{figure*}

\begin{table*}%
  \begin{center}%
    \caption{Second table.}%
    \label{tab:Dsecond}%
    \subfloat[Two subone.\label{tab:DsecondA}]{\figbox{Two subone}}
    \qquad
    \subfloat[Two subtwo.\label{tab:DsecondB}]{\figbox{Two subtwo}}\\
    \listsubcaptions
%
    \setcaptype{figure}%
    \subfloat[Three subone.\label{fig:DthirdA}]{\figbox{Three subone}}
    \qquad
    \subfloat[Three subtwo.\label{fig:DthirdB}]{\figbox{Three subtwo}}\\[-10pt]
    \caption{Third figure.}%
    \label{fig:Dthird}%
%
    \setcaptype{table}%
    \caption{Third table.}%
    \label{tab:Dthird}%
    \subfloat[Three subone.\label{tab:DthirdA}]{\figbox{Three subone}}
    \qquad
    \subfloat[Three subtwo.\label{tab:DthirdB}]{\figbox{Three subtwo}}\\
  \end{center}%
\end{table*}


\subsection{Mixed figures and tables with {\bf table} and {\bf subtable}
            captions at top}
\captionsetup[figure]{position=bottom}
%\setcounter{subfigure}{0}
\captionsetup[subfigure]{position=bottom}
\captionsetup[table]{position=top}
%\setcounter{subtable}{0}
\captionsetup[subtable]{position=top}

Figure~\ref{fig:Efirst}[\pageref{fig:Efirst}] has two subfigures
\ref{fig:EfirstA}[\pageref{fig:EfirstA}] and
\ref{fig:EfirstB}[\pageref{fig:EfirstB}].
%
Table~\ref{tab:Efirst}[\pageref{tab:Efirst}] has two subtables
\ref{tab:EfirstA}[\pageref{tab:EfirstA}] and
\ref{tab:EfirstB}[\pageref{tab:EfirstB}].
%
Figure~\ref{fig:Esecond}[\pageref{fig:Esecond}] has two subfigures
\ref{fig:EsecondA}[\pageref{fig:EsecondA}] and
\ref{fig:EsecondB}[\pageref{fig:EsecondB}].
%
Figure~\ref{fig:Ethird}[\pageref{fig:Ethird}] has two subfigures
\ref{fig:EthirdA}[\pageref{fig:EthirdA}] and
\ref{fig:EthirdB}[\pageref{fig:EthirdB}].
%
Table~\ref{tab:Esecond}[\pageref{tab:Esecond}] has two subtables
\ref{tab:EsecondA}[\pageref{tab:EsecondA}] and
\ref{tab:EsecondB}[\pageref{tab:EsecondB}].
%
Table~\ref{tab:Ethird}[\pageref{tab:Ethird}] has two subtables
\ref{tab:EthirdA}[\pageref{tab:EthirdA}] and
\ref{tab:EthirdB}[\pageref{tab:EthirdB}].
%

\begin{figure*}%
  \begin{center}%
    \subfloat[One subone.\label{fig:EfirstA}]{\figbox{One subone}}
    \qquad
    \subfloat[One subtwo.\label{fig:EfirstB}]{\figbox{One subtwo}}\\[-10pt]
    \caption{First figure.}%
    \label{fig:Efirst}%
%
    \setcaptype{table}%
    \caption{First table.}%
    \label{tab:Efirst}%
    \subfloat[One subone.\label{tab:EfirstA}]{\figbox{One subone}}
    \qquad
    \subfloat[One subtwo.\label{tab:EfirstB}]{\figbox{One subtwo}}\\
    \listsubcaptions
%
    \setcaptype{figure}%
    \subfloat[Two subone.\label{fig:EsecondA}]{\figbox{Two subone}}
    \qquad
    \subfloat[Two subtwo.\label{fig:EsecondB}]{\figbox{Two subtwo}}\\[-10pt]
    \caption{Second figure.}%
    \label{fig:Esecond}%
  \end{center}%
\end{figure*}

\begin{table*}%
  \begin{center}%
    \caption{Second table.}%
    \label{tab:Esecond}%
    \subfloat[Two subone.\label{tab:EsecondA}]{\figbox{Two subone}}
    \qquad
    \subfloat[Two subtwo.\label{tab:EsecondB}]{\figbox{Two subtwo}}\\
    \listsubcaptions
%
    \setcaptype{figure}%
    \subfloat[Three subone.\label{fig:EthirdA}]{\figbox{Three subone}}
    \qquad
    \subfloat[Three subtwo.\label{fig:EthirdB}]{\figbox{Three subtwo}}\\[-10pt]
    \caption{Third figure.}%
    \label{fig:Ethird}%
%
    \setcaptype{table}%
    \caption{Third table.}%
    \label{tab:Ethird}%
    \subfloat[Three subone.\label{tab:EthirdA}]{\figbox{Three subone}}
    \qquad
    \subfloat[Three subtwo.\label{tab:EthirdB}]{\figbox{Three subtwo}}\\
  \end{center}%
\end{table*}

\end{document}
