# Supplementary material for: Ion Impact Induced Ultrafast Electron Dynamics in Correlated Materials and Finite Graphene Clusters
Source: arXiv:1808.07868 source file (2018-09-19)
Supplement: Supplementary file 5 [file test4.tex]

%% test4.tex
%%
%% This is file `test4.tex', one of a set of several test/example files
%% in the `subfig' package.
%%
%% Copyright © 2003, 2004, 2005 Steven Douglas Cochran.
%% 
%% This work (the subfig package) may be distributed and/or modified 
%% under the conditions of the LaTeX Project Public License, either 
%% version 1.3 of this license or (at your option) any later version.
%% The latest version of this license is in
%%   http://www.latex-project.org/lppl.txt
%% and version 1.3 or later is part of all distributions of LaTeX
%% version 2003/12/01 or later.
%%
%% This work has the LPPL maintenance status "author-maintained".
%% 
%% This Current Maintainer of this work is Steven Douglas Cochran.
%%
%% This work consists of all files listed under "MANIFEST" in the
%% README file distributed with the subfig package.

\documentclass{article}
\usepackage[config=altsf]{subfig}
% option for use with pdflatex
%\usepackage{hyperref}
%\usepackage[draft]{hyperref}
\usepackage[pdftex]{hyperref}
\usepackage{makeidx}
\captionsetup[subfigure]{subrefformat=parens}

% reset the index environment to print the index section in the TOC.
\makeatletter
\renewenvironment{theindex}{%
    \if@twocolumn
      \@restonecolfalse
    \else
      \@restonecoltrue
    \fi
    \columnseprule \z@
    \columnsep 35\p@
    \twocolumn[\section{\indexname}]%
    \@mkboth{\MakeUppercase\indexname}{\MakeUppercase\indexname}%
    \thispagestyle{plain}%
    \parindent\z@
    \parskip\z@ \@plus .3\p@\relax
    \let\item\@idxitem
  }{%
    \if@restonecol
      \onecolumn
    \else
      \clearpage
    \fi
  }
  \renewcommand\abstract[1]{%
    \def\@abstract{%
      \centerline{{\large\bf Abstract}}
      \noindent
      #1}}
  \renewcommand\@maketitle{%
    \newpage
    \null\vfil
    \vskip 60\p@
    \begin{center}%
      {\LARGE \@title \par}%
      \vskip 3em%
      {\large
       \lineskip .75em%
       \begin{tabular}[t]{c}%
         \@author
       \end{tabular}\par}%
      \vskip 1.5em%
      {\large \@date \par}% 
    \end{center}%
    \vskip 2.5em%
    \@abstract
    \vfil\null}%
\makeatother

\makeindex

\begin{document}

\title{Subfig Package Test Program Four}
\author{Steven Douglas Cochran\\
        Digital Mapping Laboratory\\
        School of Computer Science\\
        Carnegie-Mellon University\\
        5000 Forbes Avenue\\
        Pittsburgh, PA 15213-3890\\
        USA}
\date{21 December 2003}
\abstract{This test checks the interaction with the {\bf hyperref}
  package and the use of the {\bf altsf.cfg} configuration file.}
\maketitle
\clearpage

\tableofcontents
\clearpage
\setcounter{lofdepth}{2}
\listoffigures
\clearpage

\section{Test of subfigure}

There is a \index{test}test \index{figure}figure \ref{fig:test} with
\index{subfigure}subfigures \ref{fig:testsub1} and \ref{fig:testsub2}.

Also referenced with \ref{fig:test}\subref{fig:testsub1} and
\ref{fig:test}\subref{fig:testsub2}.

One other way to reference these is with the starred subref command.
For example, with \subref*{fig:testsub1} and \subref*{fig:testsub2}.

The chief purpose of this test is to check and verify the interaction
between the subfigure package and the hyperref package.


\begin{figure}[!ht]
    \centering
    \unitlength .5cm
    \subfigure[SubFig1]
    { \label(SubFig1){fig:testsub1}
        \begin{picture}(10,10)
            \put(0,0){\line(1,1){10}}
        \end{picture}
    }
    \qquad
    \subfigure[SubFig2]
    { \label{fig:testsub2}
        \begin{picture}(10,10)
            \put(0,10){\line(1,-1){10}}
        \end{picture}
    }
    \caption{Testfigures}
    \label{fig:test}
\end{figure}

\clearpage

\printindex

\end{document}
